# Supplementary material for: AB-Training: A Communication-Efficient Approach for Distributed Low-Rank Learning
Source: arXiv:2405.01067 source file (2024-06-30)
Supplement: Supplementary file 1 [file supp.tex]

\newcommand{\appendix}{

}
